# Supplementary material for: Deep Structured Reactive Planning
Source: arXiv:2101.06832 source file (2021-04-29)
Supplement: Supplementary file 1 [file abstract.tex]

% !TEX root = ./root.tex
\begin{abstract}
In the supplementary materials, we provide additional model information regarding our joint structured model: this includes architectural details as well as discussion on various model properties. We then provide more details about the experimental setup of the PRECOG baseline \cite{rhinehart_precog}. We provide numerous additional experimental results, consisting of three components: 1) we demonstrate the effects of varying weights on the planning costs 2) we show that we can flexibly interpolate between the reactive/non-reactive objectives within our model, and that metrics vary accordingly as we shift along the spectrum; and 3) we present numerous additional qualitative results highlighting the difference between non-reactive/reactive models. 
%and that interpolation can be a useful means of finding the right balance between aggressive and passive behavior if necessary. 
\end{abstract}

% Both the reactive and standard non-reactive objectives are based on a powerful deep energy-based model allowing us to explicitly model unary and pairwise interactions between actors. We demonstrate multiple key results: 1) that with validated hyperparameters, the reactive model outperforms the non-reactive model in simulated interactive scenarios, 2) that we can flexibly interpolate between reactive/non-reactive behavior to tradeoff goal completion/collision if necessary, 3) that our joint structured model outperforms state-of-the-art on standard prediction datasets. In future work, we plan on exploring how to better learn how to better adapt reactivity to the given scenario, potentially in a reinforcement learning setting.  
