# Supplementary material for: Deep Structured Reactive Planning
Source: arXiv:2101.06832 source file (2021-04-29)
Supplement: Supplementary file 2 [file results_exp.tex]

\section{Additional Experiment Details}
