# Supplementary material for: Deep Structured Reactive Planning
Source: arXiv:2101.06832 source file (2021-04-29)
Supplement: Supplementary file 3 [file root.tex]

%%%%%%%%%%%%%%%%%%%%%%%%%%%%%%%%%%%%%%%%%%%%%%%%%%%%%%%%%%%%%%%%%%%%%%%%%%%%%%%%
%2345678901234567890123456789012345678901234567890123456789012345678901234567890
%        1         2         3         4         5         6         7         8

\documentclass[letterpaper, 10 pt, conference]{ieeeconf}  % Comment this line out if you need a4paper

\IEEEoverridecommandlockouts                              % This command is only needed if 
                                                          % you want to use the \thanks command

\overrideIEEEmargins                                      % Needed to meet printer requirements.

%In case you encounter the following error:
%Error 1010 The PDF file may be corrupt (unable to open PDF file) OR
%Error 1000 An error occurred while parsing a contents stream. Unable to analyze the PDF file.
%This is a known problem with pdfLaTeX conversion filter. The file cannot be opened with acrobat reader
%Please use one of the alternatives below to circumvent this error by uncommenting one or the other
%\pdfobjcompresslevel=0
%\pdfminorversion=4

% See the \addtolength command later in the file to balance the column lengths
% on the last page of the document

% The following packages can be found on http:\\www.ctan.org
%\usepackage{graphics} % for pdf, bitmapped graphics files
%\usepackage{epsfig} % for postscript graphics files
%\usepackage{mathptmx} % assumes new font selection scheme installed
%\usepackage{times} % assumes new font selection scheme installed
%\usepackage{amsmath} % assumes amsmath package installed
%\usepackage{amssymb}  % assumes amsmath package installed

\title{\LARGE \bf
Deep Structured Reactive Planning - Supplementary Materials
}

\author{Jerry Liu$^{1}$ and Wenyuan Zeng $^{1,2}$ and Raquel Urtasun $^{1,2}$ and Ersin Yumer$^{1}$% <-this % stops a space
	\thanks{$^{1}$ Uber ATG. Correspondence to: {\tt\small \{jerryl, wenyuan, urtasun, yumer\}@uber.com}}%
	\thanks{$^{2}$ University of Toronto}%
}

\usepackage{subcaption} 
\usepackage{cite}
\usepackage{amsmath,amssymb,amsfonts}
\usepackage{algorithmic}
\usepackage{graphicx}
\usepackage{textcomp}
\usepackage{xcolor}
\usepackage{booktabs} 
\usepackage{multirow}
\usepackage{pbox}
\usepackage{hyperref}
\usepackage{overpic}
\def\BibTeX{{\rm B\kern-.05em{\sc i\kern-.025em b}\kern-.08em
		T\kern-.1667em\lower.7ex\hbox{E}\kern-.125emX}}
\begin{document}

\newcommand{\bw}{{\mathbf{w}}}
\newcommand{\by}{{\mathbf{y}}}
\newcommand{\cY}{{\mathcal{Y}}}
\newcommand{\cX}{{\mathcal{X}}}
\newcommand{\Exp}{{\mathbb{E}}}

\newcommand{\raquel}[1]{\textcolor{red}{Raquel: #1}}
\newcommand{\wenyuan}[1]{\textcolor{blue}{Wenyuan: #1}}
\newcommand{\jerry}[1]{\textcolor{purple}{Jerry: #1}}
\newcommand{\ersin}[1]{\textcolor{cyan}{Ersin: #1}}

\maketitle
\thispagestyle{empty}
\pagestyle{empty}

% !TEX root = ./root.tex
\begin{abstract}
In the supplementary materials, we provide additional model information regarding our joint structured model: this includes architectural details as well as discussion on various model properties. We then provide more details about the experimental setup of the PRECOG baseline \cite{rhinehart_precog}. We provide numerous additional experimental results, consisting of three components: 1) we demonstrate the effects of varying weights on the planning costs 2) we show that we can flexibly interpolate between the reactive/non-reactive objectives within our model, and that metrics vary accordingly as we shift along the spectrum; and 3) we present numerous additional qualitative results highlighting the difference between non-reactive/reactive models. 
%and that interpolation can be a useful means of finding the right balance between aggressive and passive behavior if necessary. 
\end{abstract}

% Both the reactive and standard non-reactive objectives are based on a powerful deep energy-based model allowing us to explicitly model unary and pairwise interactions between actors. We demonstrate multiple key results: 1) that with validated hyperparameters, the reactive model outperforms the non-reactive model in simulated interactive scenarios, 2) that we can flexibly interpolate between reactive/non-reactive behavior to tradeoff goal completion/collision if necessary, 3) that our joint structured model outperforms state-of-the-art on standard prediction datasets. In future work, we plan on exploring how to better learn how to better adapt reactivity to the given scenario, potentially in a reinforcement learning setting.  

\input{architecture.tex}
\input{model_properties.tex}
\input{results_varyhyp.tex}
\input{results_interpolate.tex}
\input{results_precog.tex}
\input{results_vis.tex}

\clearpage
\bibliographystyle{splncs04}
\bibliography{egbib}

\end{document}
